# Supplementary material for: U-shaped and Inverted-U Scaling behind Emergent Abilities of Large Language Models
Source: arXiv:2410.01692 source file (2025-02-12)
Supplement: Supplementary file 1 [file code_line_description_phenomenon.tex]

\begin{figure*}[t]
  \centering
  \begin{subfigure}{0.48\linewidth}
    \includegraphics[width=\textwidth]{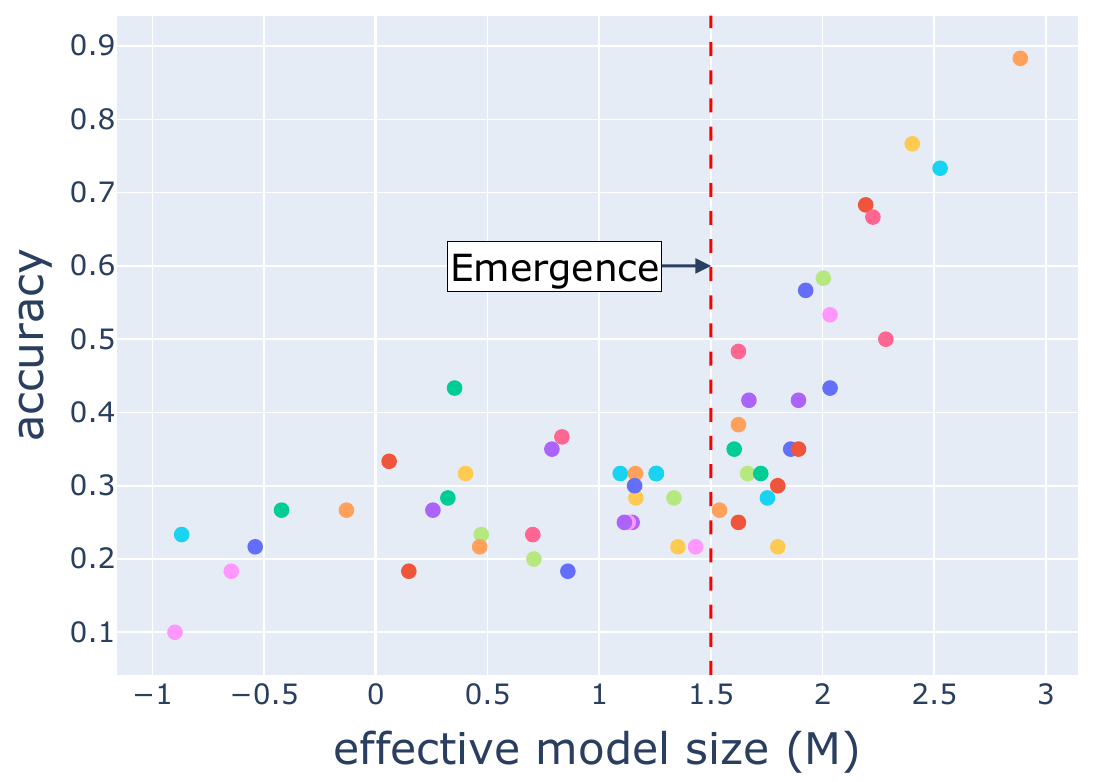}
    \caption{Accuracy vs. log compute (M).}
    \label{subfig: code_line_description accuracy}
  \end{subfigure}
  \hfill
  \begin{subfigure}{0.48\linewidth}
    \includegraphics[width=\textwidth]{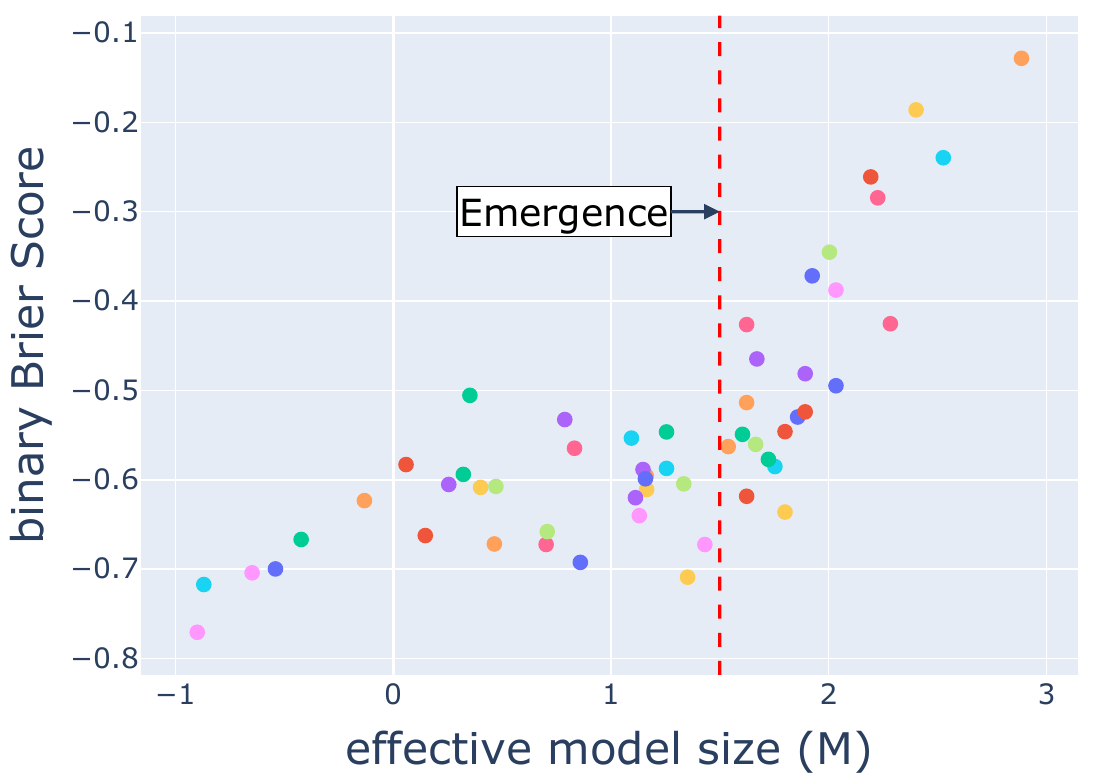}
    \caption{TC Brier Score vs. log compute (M).}
    \label{subfig: code_line_description brier}
  \end{subfigure}
  \hfill
  \begin{subfigure}{0.9\linewidth}
    \includegraphics[width=\textwidth]{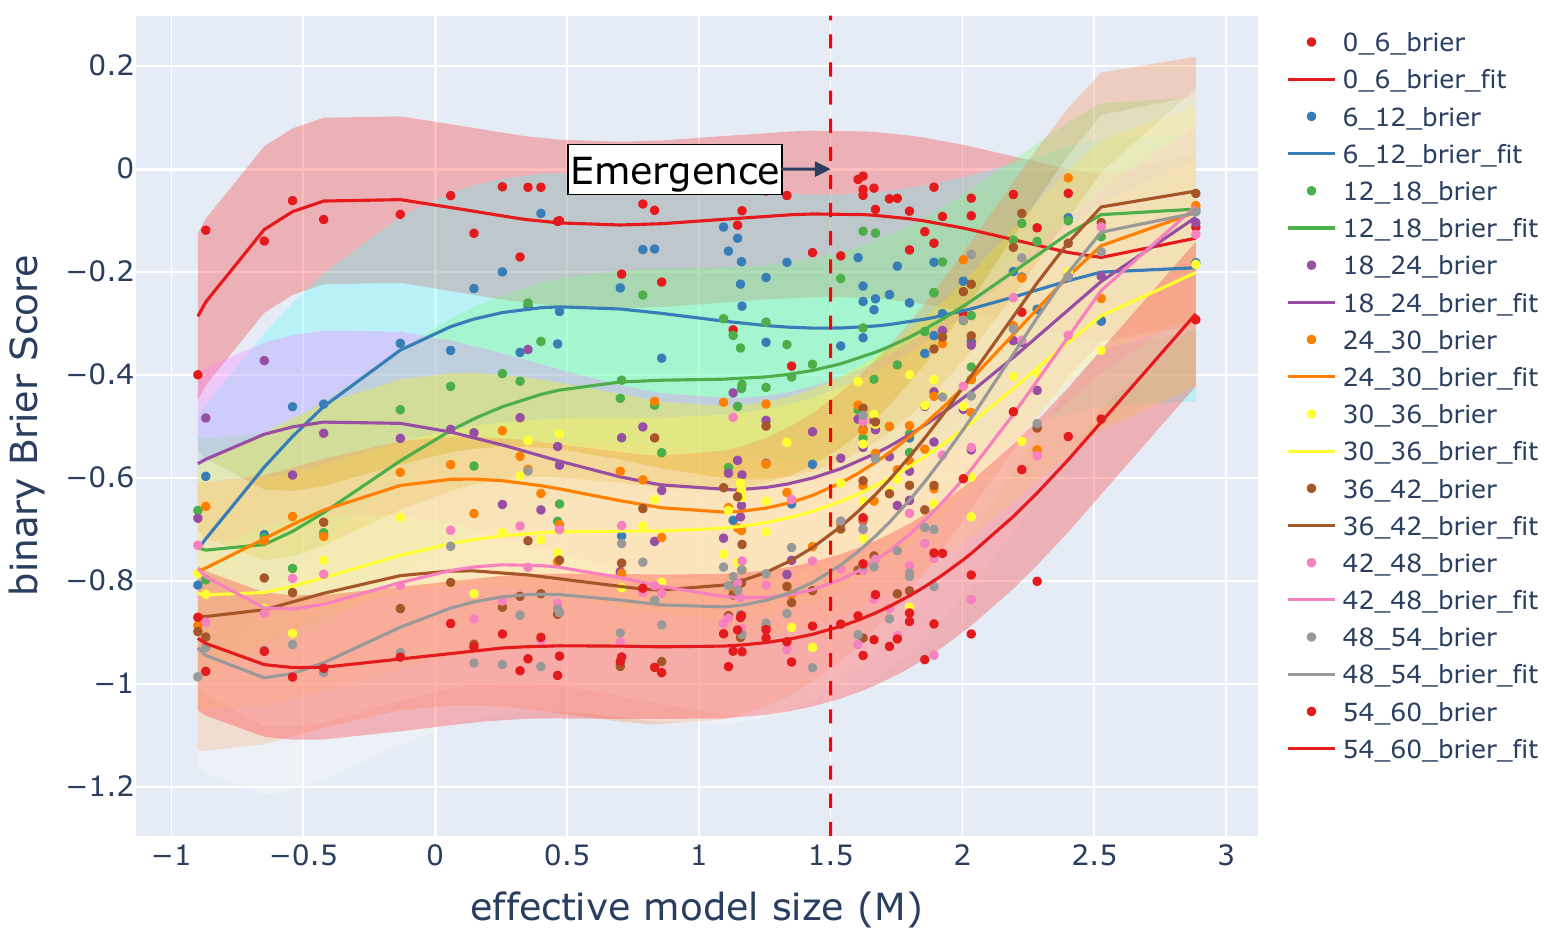}
    \caption{U-Shaped and inverted-U scaling}
    \label{subfig: code_line_description phenomenon}
  \end{subfigure}
  \caption{The accuracy, TC Brier Score, U-Shaped and inverted-U scaling on the code line description dataset in BIG-bench~\citep{srivastava2023beyond}.}
  \label{fig: code_line_description phenomenon}
\end{figure*}
